# Supplementary material for: Modeling Live Video Streaming: Real-Time Classification, QoE Inference, and Field Evaluation
Source: arXiv:2112.02637 source file (2021-12-05)
Supplement: Supplementary file 1 [file appendix.tex]

%%%
%%% If your work has an appendix, this is the place to put it.

\appendix
\section{Buffer Estimation Pseudo-Algorithm}\label{sec:apdx}
\begin{algorithm}
	\caption{Predict Buffer Stall}
		\DontPrintSemicolon % Some LaTeX compilers require you to use \dontprintsemicolon instead
		\SetNoFillComment
		\Parameter{$Buf_{min}, Seg_{dur}$}
		\KwData{\textit{Chunks} detected on network $\{c_1,c_2, \ldots, c_n\}$}
		\KwOut{Estimated buffer health}
		$b \gets 0$ \Comment*[r]{Tracks current buffer value}
		$t \gets 0$ \Comment*[r]{Tracks endTime of last chunk}
		\For{each network chunk c} {
			b  += $Seg_{dur}$   \Comment*[r]{Increment buffer by duration of each segment}
			\If{$b <= Buf_{min}$}  {
				$t  = c.EndTime$\;
				\Continue  \Comment*[r]{Wait until video starts playing}
			}
			b --= $c.EndTime - t$ \Comment*[r]{Decrement buffer by time elapsed}
			\If{$b <= 0$}{
				$b = 0$\Comment*[r]{Stall detected}
			}
		}
\end{algorithm}
